# Supplementary material for: Digging Into Self-Supervised Learning of Feature Descriptors
Source: arXiv:2110.04773 source file (2021-10-10)
Supplement: Supplementary file 4 [file fig_inloc_r2d2.tex]

\begin{figure*}[t!]
  \centering
    \includegraphics[width=1\linewidth]{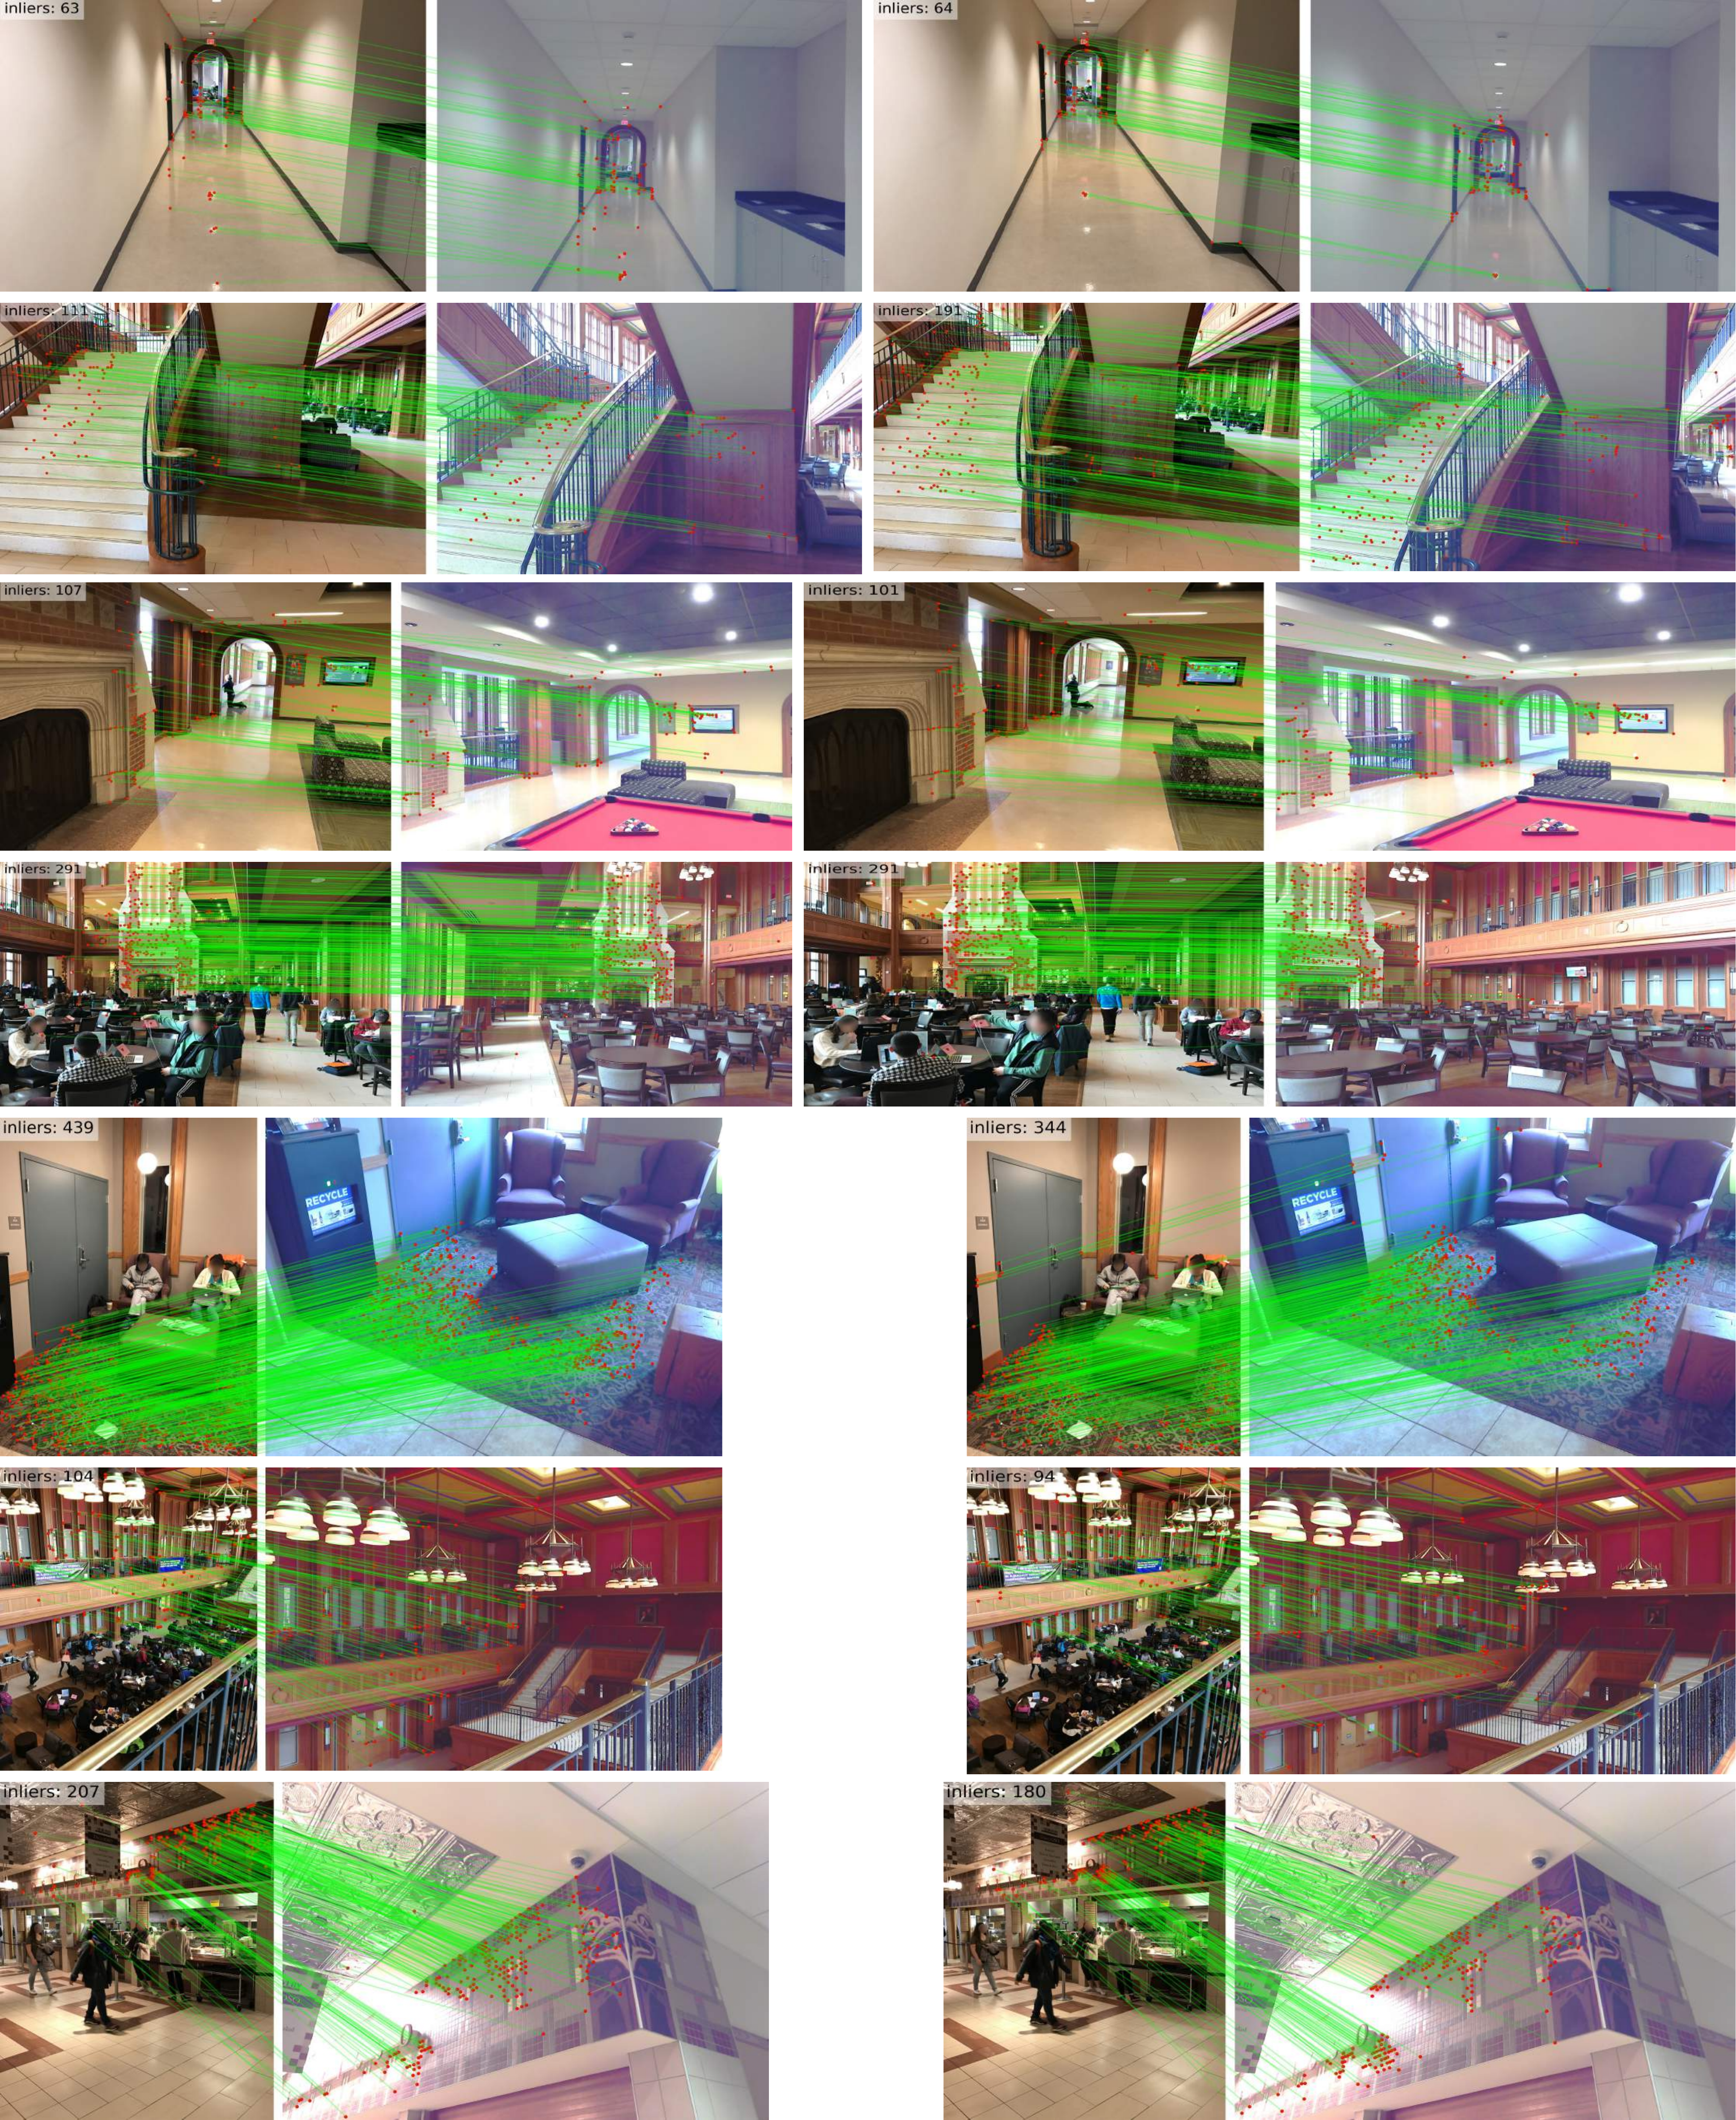}
 \caption{\textbf{Example correspondences} produced by our method (left) and its supervised counterpart,~\ie R2D2~\cite{Revaud2019R2D2} (right), on queries of InLoc~\cite{Taira2018InLoc}}  
 \label{fig:supp_inloc_r2d2}
\end{figure*}
